# Supplementary material for: There is Something Beyond the Twitter Network
Source: arXiv:1611.09387 source file (2016-11-28)
Supplement: Supplementary file 1 [file appendix.tex]

\begin{appendices}

\todo{remove sample appendix}
\section{Rdag Has Approximately Uniform Distribution of Degrees} \label{bin_un}

\end{appendices}
